# Supplementary material for: Differentiable Cyclic Causal Discovery Under Unmeasured Confounders
Source: arXiv:2508.08450 source file (2026-01-23)
Supplement: Supplementary file 1 [file supp.tex]

\documentclass{article}

\usepackage{xr}
\externaldocument{neurips_2025}

\usepackage[nonatbib]{neurips_2025}

\usepackage[utf8]{inputenc} % allow utf-8 input
\usepackage[T1]{fontenc}    % use 8-bit T1 fonts
\usepackage{hyperref}       % hyperlinks
\usepackage{url}            % simple URL typesetting
\usepackage{booktabs}       % professional-quality tables
\usepackage{amsfonts}       % blackboard math symbols
\usepackage{nicefrac}       % compact symbols for 1/2, etc.
\usepackage{microtype}      % microtypography
\usepackage{xcolor}         % colors
\usepackage{amsmath, amssymb, amsthm, bm, amsfonts}
\usepackage{tikz}
\usepackage{algorithm}
\usepackage{algpseudocode}
\usepackage{apptools}
\usepackage{subcaption}
\usepackage{wrapfig}
\usepackage{enumitem}
\usepackage[numbers]{natbib}
\bibliographystyle{unsrtnat}

\input{macros}

\AtAppendix{\counterwithin{define}{section}}

%%%%%%%%%%%%%%%%%%%%%%%%%%%%%%%%%%%%%%%%%%%%%%%%%%%%%%%%%%
% Remember to remove the following lines when combining the appendix with the main document
%%%%%%%%%%%%%%%%%%%%%%%%%%%%%%%%%%%%%%%%%%%%%%%%%%%%%%%%%%

\begin{document}

\appendix
\include{appendix}

\bibliography{references}

\end{document}
